# Supplementary material for: Kernel Interpolation with Sparse Grids
Source: arXiv:2305.14451 source file (2023-05-23)
Supplement: Supplementary file 1 [file supplement.tex]

\clearpage
%%%%%%%%%%%%%%%%%%%%%%%%%%%%%%%%%%%%%%%%%%%%%%%%%%%%%%%%%%%%
